# Supplementary material for: Conformal Prediction under Levy-Prokhorov Distribution Shifts: Robustness to Local and Global Perturbations
Source: arXiv:2502.14105 source file (2025-05-19)
Supplement: Supplementary file 1 [file imgnet_plot.tex]

\documentclass[tikz,100pt]{standalone}
\usepackage{amsmath,amsfonts,amssymb}
\usepackage{xcolor}
\usepackage{tikz}
\usetikzlibrary{positioning}
\usetikzlibrary{arrows,calc}
\usepackage{pgfplots}

\newdimen\iwidth
\newdimen\iheight
\newdimen\vsp
\newdimen\hsp

% \usepackage{siunitx}
% \sisetup{round-precision=4,round-mode=figures,scientific-notation=true}

\tikzstyle{every node}=[font=\footnotesize]
\usetikzlibrary{spy}
\usetikzlibrary{decorations.pathreplacing}
\tikzstyle{label}=[color=white,
fill=gray,opacity=.9,
rectangle,rounded corners,
draw,minimum height=0.5cm]

\begin{document}
	\pagestyle{empty}
	
	\begin{tikzpicture}[scale=1] 
		\newcommand{\image}[1]{\includegraphics[width=0.48\linewidth, clip=true]{#1}}
        
		\node[] (A) at  (0,0) {\image{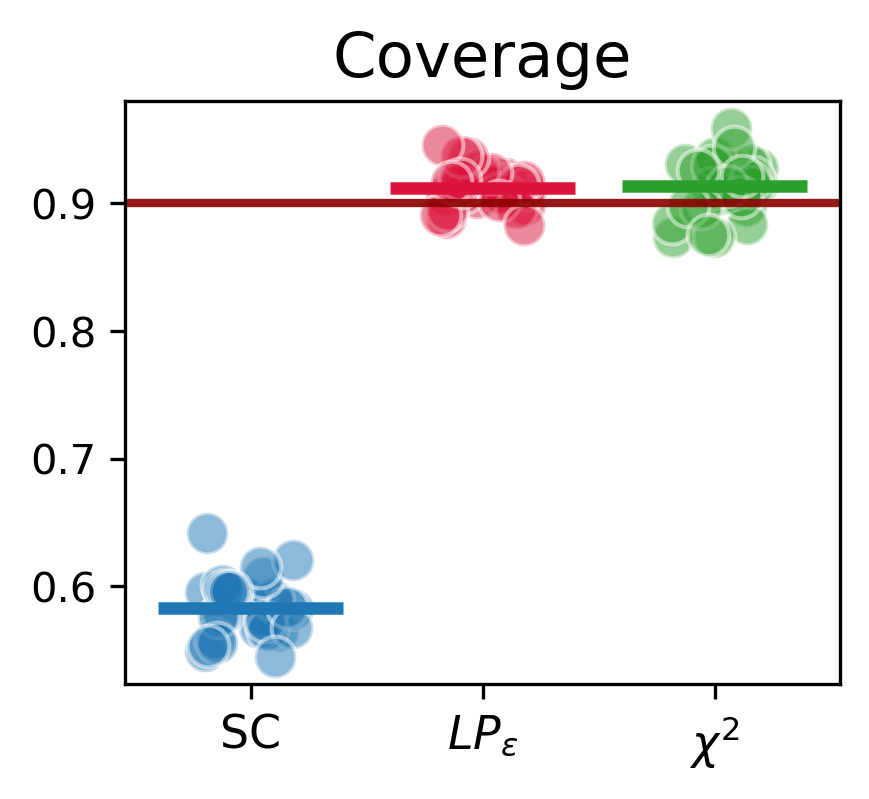}};%
        
    	   \node[right = of A, xshift=-40pt] (B) {\image{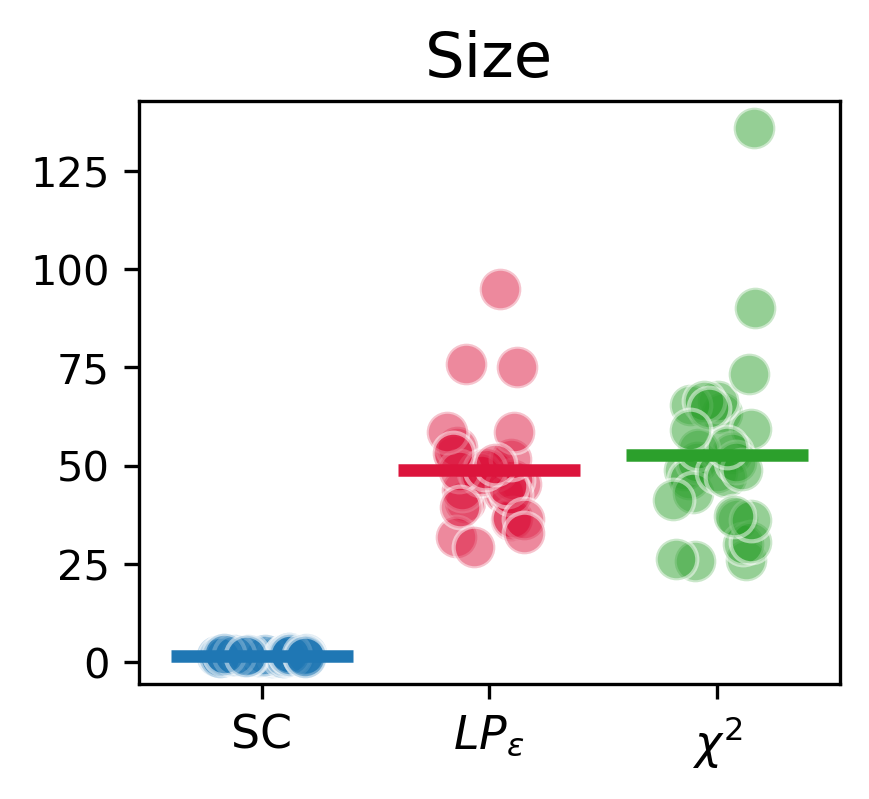}};%
           
           % \node[label, above= of A, font=\Large, xshift=86pt, yshift=-30pt] {(p=0.05, u=3.0)};%
            \node[label, left= of A, rotate=90, font=\Large, xshift=30.5pt, yshift=-20pt] {ImageNet};%
\end{tikzpicture}
\end{document}
